# Supplementary material for: Few-Shot Scene Adaptive Crowd Counting Using Meta-Learning
Source: arXiv:2002.00264 source file (2020-06-19)
Supplement: Supplementary file 1 [file tab_meta_supplementary.tex]

% K=1 and K=5

\begin{table*}[!ht]
  \centering
  \small
  \resizebox{0.9\textwidth}{!}{%

\begin{tabular}{cccccccc}
\Xhline{2\arrayrulewidth}
\multirow{2}{*}{\textbf{Target}} & \multirow{2}{*}{\textbf{Methods}} & \multicolumn{3}{c}{\textbf{1-shot (K=1)}}                                         & \multicolumn{3}{c}{\textbf{5-shot (K=5)}}                                         \\ 
                                 &                                   & \multicolumn{1}{c}{MAE}                       & \multicolumn{1}{c}{RMSE}                       & \multicolumn{1}{c}{MDE}                        & \multicolumn{1}{c}{MAE}                       & \multicolumn{1}{c}{RMSE}                       & \multicolumn{1}{c}{MDE}                        \\ \cline{1-8} 
\multirow{4}{*}{Scene 1}         
& Meta-LSTM~\cite{ravi2016optimizationmethod} & 4.52 $\pm$ {\footnotesize 1.06}           & 5.95 $\pm$ {\footnotesize 1.62}           & 0.40 $\pm$ {\footnotesize 0.08}           & 3.66 $\pm$ {\footnotesize 0.85}           & 4.64 $\pm$ {\footnotesize 1.30}           & 0.39 $\pm$ {\footnotesize 0.10}           \\ 
& Reptile~\cite{nichol2018first}            & 4.99 $\pm$ {\footnotesize 0.46}           & 7.08 $\pm$ {\footnotesize 1.09}  & 0.47 $\pm$ {\footnotesize 0.123}           & 3.38 $\pm$ {\footnotesize 0.59}           & 4.38 $\pm$ {\footnotesize 0.63}          & 0.36 $\pm$ {\footnotesize 0.112}   \\ %\cdashline{2-8}
& \textbf{Ours w/o ROI}             & 3.47 $\pm$ {\footnotesize 0.01}           & \textbf{4.19 $\pm$ {\footnotesize 0.01}}  & 0.50 $\pm$ {\footnotesize 0.007}           & 3.42 $\pm$ {\footnotesize 0.03}           & 4.81 $\pm$ {\footnotesize 0.007}          & \textbf{0.29 $\pm$ {\footnotesize 0.004}}   \\ 

& \textbf{Ours w/ ROI}            & \textbf{3.19 $\pm$ {\footnotesize 0.03}}  & 4.30 $\pm$ {\footnotesize 0.07}           & \textbf{0.38 $\pm$ {\footnotesize 0.03}}   & \textbf{3.05 $\pm$ {\footnotesize 0.06}}  & \textbf{4.19 $\pm$ {\footnotesize 0.15}}  & 0.31 $\pm$ {\footnotesize 0.08}            \\ \hline

\multirow{4}{*}{Scene 2}          
& Meta-LSTM~\cite{ravi2016optimizationmethod}                        & 19.09 $\pm$ {\footnotesize 3.54}           & 26.42 $\pm$ {\footnotesize 5.11}           & 0.22 $\pm$ {\footnotesize 0.01}           & 18.89 $\pm$ {\footnotesize 1.87}           & 26.35 $\pm$ {\footnotesize 2.61}           & 0.160 $\pm$ {\footnotesize 0.014}           \\ & Reptile~\cite{nichol2018first}             & 21.51 $\pm$ {\footnotesize 0.45}           & 25.85 $\pm$ {\footnotesize 0.48}  & 0.30 $\pm$ {\footnotesize 0.062}           & 14.52 $\pm$ {\footnotesize 3.11}           & 20.46 $\pm$ {\footnotesize 4.29}          & 0.14 $\pm$ {\footnotesize 0.049}   \\ %\cline{2-8}
& \textbf{Ours w/o ROI}             & 12.05 $\pm$ {\footnotesize 0.74}          & 16.62 $\pm$ {\footnotesize 1.10}          & 0.11 $\pm$ {\footnotesize 0.007}           & 11.41 $\pm$ {\footnotesize 0.54}          & 15.35 $\pm$ {\footnotesize 0.51}          & 0.11 $\pm$ {\footnotesize 0.015}           \\
& \textbf{Ours w/ ROI}            & \textbf{11.17 $\pm$ {\footnotesize 1.01}} & \textbf{15.50 $\pm$ {\footnotesize 1.18}} & \textbf{0.11 $\pm$ {\footnotesize 0.012}}  & \textbf{10.73 $\pm$ {\footnotesize 0.36}} & \textbf{14.95 $\pm$ {\footnotesize 0.60}} & \textbf{0.10 $\pm$ {\footnotesize 0.003}}  \\ \hline

\multirow{4}{*}{Scene 3}         
& Meta-LSTM~\cite{ravi2016optimizationmethod}                        & 24.66 $\pm$ {\footnotesize 1.13}           & 33.54 $\pm$ {\footnotesize 1.22}           & 0.29 $\pm$ {\footnotesize 0.011}           & 24.24 $\pm$ {\footnotesize 0.95}           & 29.38 $\pm$ {\footnotesize 1.15}           & 0.27 $\pm$ {\footnotesize 0.008}           \\ 
& Reptile~\cite{nichol2018first}             & 14.14 $\pm$ {\footnotesize 1.68}           & 18.04 $\pm$ {\footnotesize 1.71}  & 0.156 $\pm$ {\footnotesize 0.015}           & 9.37 $\pm$ {\footnotesize 1.30}           & 12.04 $\pm$ {\footnotesize 1.27}          & 0.123 $\pm$ {\footnotesize 0.026}   \\ %\cline{2-8}

& \textbf{Ours w/o ROI}             & 8.15 $\pm$ {\footnotesize 0.17}           & 11.04 $\pm$ {\footnotesize 0.42}          & \textbf{0.09 $\pm$ {\footnotesize 0.04}}  & 8.31 $\pm$ {\footnotesize 0.54}           & \textbf{10.75 $\pm$ {\footnotesize 0.54}} & 0.10 $\pm$ {\footnotesize 0.009}          \\
& \textbf{Ours w/ ROI}            & \textbf{8.07 $\pm$ {\footnotesize 0.23}}  & \textbf{10.92 $\pm$ {\footnotesize 0.21}} & 0.10 $\pm$ {\footnotesize 0.007}           & \textbf{8.18 $\pm$ {\footnotesize 0.24}}  & 10.96 $\pm$ {\footnotesize 0.31}          & \textbf{0.09 $\pm$ {\footnotesize 0.002}} \\ \hline

\multirow{4}{*}{Scene 4}         
& Meta-LSTM~\cite{ravi2016optimizationmethod}                        & 12.88 $\pm$ {\footnotesize 0.88}           & 15.83 $\pm$ {\footnotesize 0.9}           & 0.114 $\pm$ {\footnotesize 0.007}           & 12.03 $\pm$ {\footnotesize 0.22}           & 14.78 $\pm$ {\footnotesize 0.36}           & 0.105 $\pm$ {\footnotesize 0.002}           \\ 
& Reptile~\cite{nichol2018first}             & 12.09 $\pm$ {\footnotesize 1.28}           & 14.64 $\pm$ {\footnotesize 1.09}  & 0.106 $\pm$ {\footnotesize 0.017}           & 9.64 $\pm$ {\footnotesize 1.22}           & 12.11 $\pm$ {\footnotesize 1.34}          & 0.082 $\pm$ {\footnotesize 0.011}   \\ %\cline{2-8}
& \textbf{Ours w/o ROI}             & 9.74 $\pm$ {\footnotesize 0.09}          & 11.9 $\pm$ {\footnotesize 0.12}          & 0.084 $\pm$ {\footnotesize 0.001}           & 11.21 $\pm$ {\footnotesize 0.47}          & 16.1 $\pm$ {\footnotesize 0.45}          & 0.118 $\pm$ {\footnotesize 0.004}           \\ 
& \textbf{Ours w/ ROI}            & \textbf{9.39 $\pm$ {\footnotesize 0.26}} & \textbf{11.78 $\pm$ {\footnotesize 0.34}} & \textbf{0.07 $\pm$ {\footnotesize 0.02}}  & \textbf{9.41 $\pm$ {\footnotesize 0.21}} & \textbf{11.91 $\pm$ {\footnotesize 0.17}} & \textbf{0.08 $\pm$ {\footnotesize 0.002}}   \\ \hline

\multirow{4}{*}{Scene 5}         
& Meta-LSTM~\cite{ravi2016optimizationmethod}                        & 5.54 $\pm$ {\footnotesize 0.29}           & 9.36 $\pm$ {\footnotesize 0.35}           & 0.24 $\pm$ {\footnotesize 0.01}           & 4.68 $\pm$ {\footnotesize 0.17}           & 7.92 $\pm$ {\footnotesize 0.577}           & 0.194 $\pm$ {\footnotesize 0.002}           \\ 
& Reptile~\cite{nichol2018first}             & 5.42 $\pm$ {\footnotesize 0.32}           & 9.75 $\pm$ {\footnotesize 0.34}  & 0.27 $\pm$ {\footnotesize 0.081}           & 4.10 $\pm$ {\footnotesize 0.66}           & 7.57 $\pm$ {\footnotesize 1.20}          & 0.204 $\pm$ {\footnotesize 0.058}   \\ %\cline{2-8}
& \textbf{Ours w/o ROI}             & 4.09 $\pm$ {\footnotesize 0.01}           & 7.36 $\pm$ {\footnotesize 0.01}           & 0.196 $\pm$ {\footnotesize 0.001}           & 4.28 $\pm$ {\footnotesize 0.14}           & 7.68 $\pm$ {\footnotesize 0.60}           & 0.20 $\pm$ {\footnotesize 0.001}           \\  
& \textbf{Ours w/ ROI}            & \textbf{3.82 $\pm$ {\footnotesize 0.05}}  & \textbf{6.91 $\pm$ {\footnotesize 0.11}}  & \textbf{0.192 $\pm$ {\footnotesize 0.001}} & \textbf{3.91 $\pm$ {\footnotesize 0.26}}  & \textbf{7.18 $\pm$ {\footnotesize 0.85}}  & \textbf{0.18 $\pm$ {\footnotesize 0.001}} \\ \hline

\multirow{4}{*}{\textbf{Average}}                                    
& Meta-LSTM~\cite{ravi2016optimizationmethod}                        & 13.33 & 18.22  & 0.252 & 12.7  & 16.61 & 0.223 \\ 
& Reptile~\cite{nichol2018first}             & 11.63            & 15.07  & 0.260 & 8.20 & 11.31 & 0.181 \\ %\cline{2-8}
& \textbf{Ours w/o ROI}             & 7.5                 & 10.22                 & 0.197                  & 7.7                 & 10.93                 & 0.165                  \\ 
& \textbf{Ours w/ ROI}            & \textbf{7.12}                      & \textbf{9.88}                         & \textbf{0.172 }                          & \textbf{7.05                         } & \textbf{9.83}                           & \textbf{0.155} \\ \Xhline{2\arrayrulewidth}
\end{tabular}}
\caption{The overall results for adaptation on WorldExpo'10~\cite{zhang2015crosscounting} test set with $K = 1$ and $K = 5$ train images. We explore alterntaive optimization based meta-learning approaches such as \textit{Meta-LSTM}~\cite{ravi2016optimizationmethod} and \textit{Reptile}~\cite{nichol2018first} along with our models \textit{``Ours w/o ROI''} and \textit{``Ours w/ ROI''}. The results in bold represent the overall best result. }
\label{tab:meta_supplementary}
\end{table*}
